# Supplementary material for: Quasiperiodic gallium adlayer on i-Al-Pd-Mn
Source: arXiv:2312.12005 source file (2023-12-19)
Supplement: Supplementary file 1 [file supplementary_Ga_APM_R1_arxiv.pdf]

# Supplementary information for the manuscript entitled: "Quasiperiodic gallium adlayer on *i*-Al-Pd-Mn"

Pramod Bhakuni[1], Marian Krajčí[2,*], Sudipta Roy Barman[1,†]

[1] *UGC-DAE Consortium for Scientific Research, Khandwa Road, Indore - 452001, Madhya Pradesh, India and*

[2] *Institute of Physics, Slovak Academy of Sciences, Dúbravská cesta 9, SK-84511 Bratislava, Slovak Republic*

**The supplementary material contains Discussions I and II, one table (Table S1), ten figures (Figs. S1-S10) and two LEED mp4 video files named "Ga0.7ML" for 0.7 ML and "Ga1.2ML" for the 1.2 ML Ga coverage. The video files show a sequence of LEED patterns as a function of beam energy in the range of 30 eV <$E_p$< 180 eV at a step of 2 eV, as indicated in the bottom left corner of each pattern. The video files are uploaded separately.**

## Discussion I

The adsorption energies of the Ga clusters on the $i$-Al-Pd-Mn surface presented in the main text are compared here with the energies of the SnWF clusters [1]. The adsorption energy per atom $E_a$ is defined as $E_a$= ($E_{tot}$[Sn]$-E_{surf}$)/N+$\mu$[Sn], where $E_{surf}$ is the energy of the model $i$-Al-Pd-Mn surface representing the atomic structure of the clean quasicrystalline 5-fold surface. $E_{tot}$[Sn] is the energy of the $i$-Al-Pd-Mn surface model with the adsorbed Sn adatoms. $N_A$ is the number of adatoms in the cluster on the surface. $\mu$[Sn] is the chemical potential of Sn in the crystalline structure, $\mu$[Sn]= $-E_{cryst}$[Sn.cF8]= 3.765 eV.

TABLE S 1. Adsorption energies per atom $E_a$ [eV] of Sn clusters consisting from $N_A$ adatoms on the 5-fold $i$-Al-Pd-Mn surface.

| | Single Sn | Outer 5-Sn | WF cluster |
|---|---|---|---|
| $N_A$ | 1 | 5 | 10 |
| $E_a$ | $-1.593$ | $-0.788$ | $-0.795$ |

A single Sn atom is adsorbed in the reactive 5-Al center, as in the Ga case. The SnWF cluster consists of two pentagonal 5-Sn rings - outer and inner. In the SnWF cluster, the outer 5-Sn atoms occupy the same sites as in the outer 5-Ga cluster. At SnWF, the inner 5-Sn ring around the central Mn atom has the same orientation as the outer ring (similarly in Bi and Pb clusters). At GaWF, the outer and inner rings have opposite orientations. In the SnWF cluster, the atoms in the outer and inner rings are close together and mutually bonded. Contrary to the GaWF case, the adsorption of the SnWF cluster is stronger than the adsorption of the outer 5-fold rings only. The adsorption energy $E_a$ of the complete SnWF cluster of $-0.795$ eV is significantly larger than $E_a = -0.354$ eV of the GaWF cluster.

**Discussion II**

The adsorption energies $E_a$ calculated for a Ga adatom and clusters of Ga adatoms on crystalline Al(111) are discussed here. $E_a$ in Table I of the main text for Ga/$i$-Al-Pd-Mn represents the binding energy of the Ga adatom with respect to the binding energy of Ga in its crystalline structure, $E_{cryst}$[Ga.oP8]$= -2.934$ eV. We find that the adsorption energy $E_a$ of a single Ga adatom on the Al(111) surface is $+0.243$ eV [Fig. S10(a)]. If this central Ga adatom is surrounded by additional 6 Ga adatoms [Fig. S10(b)] then the adsorption energy of such a cluster is $E_a = -0.023$ eV. Both values are much smaller than the values in Table I, which means that the binding energy of Ga adatoms on the Al(111) surface is close to the binding energy of Ga atoms in their crystalline structure. This indicates that the reactivity of the adsorption sites on the $i$-Al-Pd-Mn surface is significantly higher.

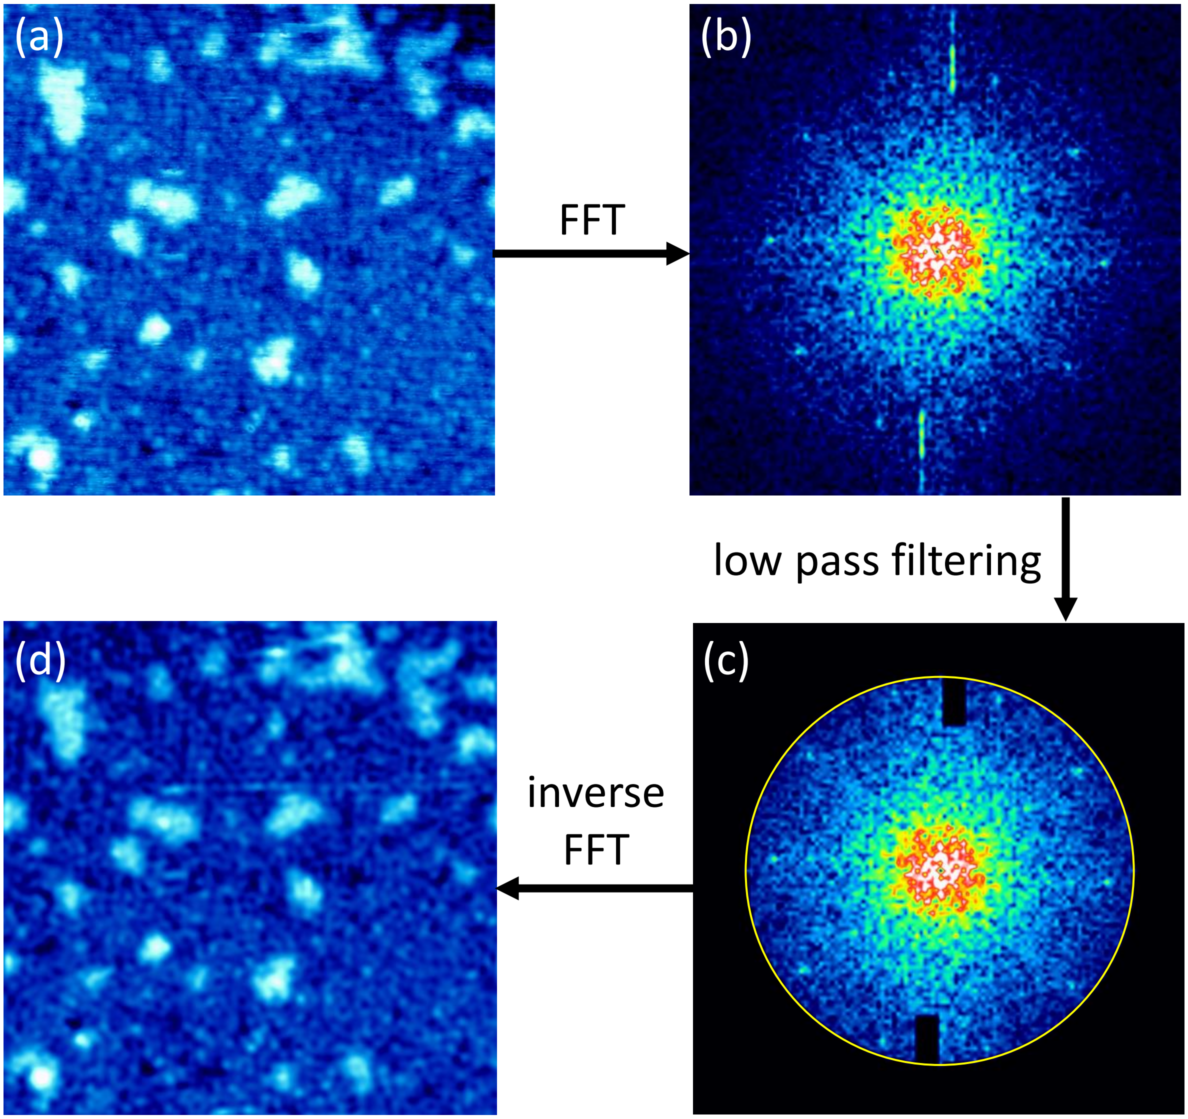


FIG. S 1. Fourier filtering procedure for (a) a raw STM image of 1.2 ML Ga/*i*-Al-Pd-Mn, where in the first step the (b) fast Fourier transform (FFT) of the STM image in panel **a** is calculated. Subsequently, (c) low pass filtering is applied to a region shown by a yellow circle that includes the central region up to the visible FFT spots for performing inverse FFT. Additionally, any evidently noisy regions are excluded, as shown by the vertical black strips. (d) The resulting low pass filtered STM image. Note that by this procedure, the image quality is improved, and in this particular case, the clearly visible, nearly horizontal noise lines in panel **a** are removed.

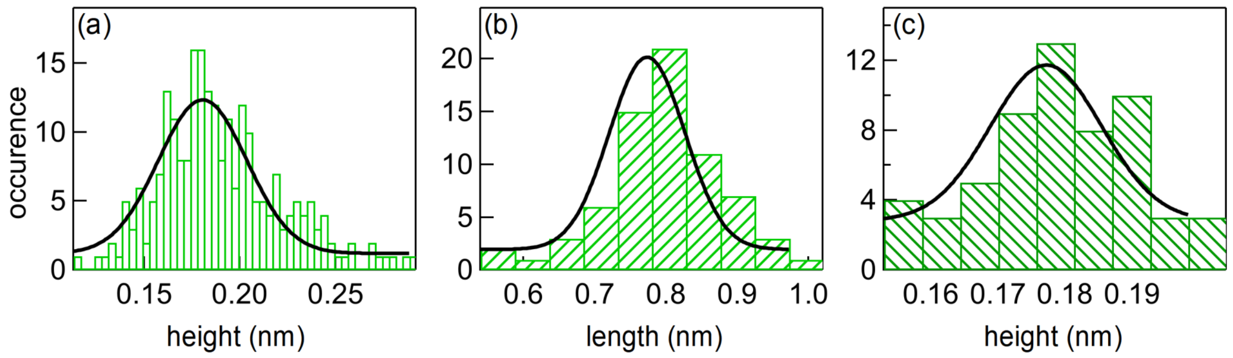


FIG. S 2. (a) Distribution of the (a) height of the Ga clusters for 0.1 ML Ga/*i*-Al-Pd-Mn, (b) the side length of the GaWF motif, and (c) the height of the Ga islands for 0.4 ML Ga/*i*-Al-Pd-Mn. The black curve represents a Gaussian fit to the distribution.

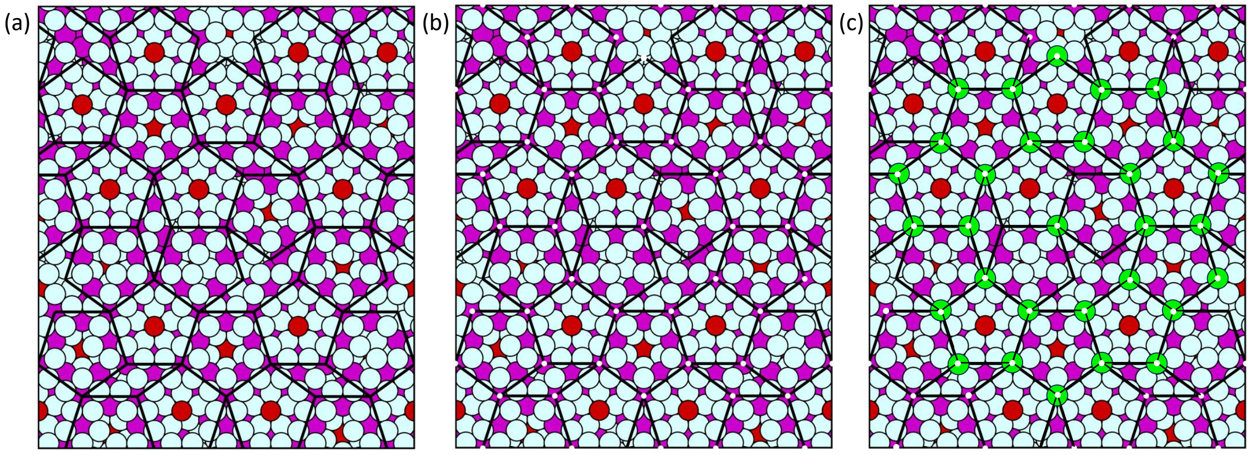


FIG. S 3. (a) The P1 tiling (black lines) shown overlaid on the atomic structure of the surface plane of 5-fold *i*-Al-Pd-Mn derived from the 5/3 approximant (5.32 nm×6.25 nm). The white, magenta, and red colored circles represent the Al, Pd, and Mn atoms, respectively. (b) Same as panel **a**, with the white dots showing all the favorable absorption positions of Ga atoms on Pd at the center of the 5-Al surface cluster. (c) A complete ring motif where all the energetically favorable sites occupied by Ga atoms (green circles) are shown.

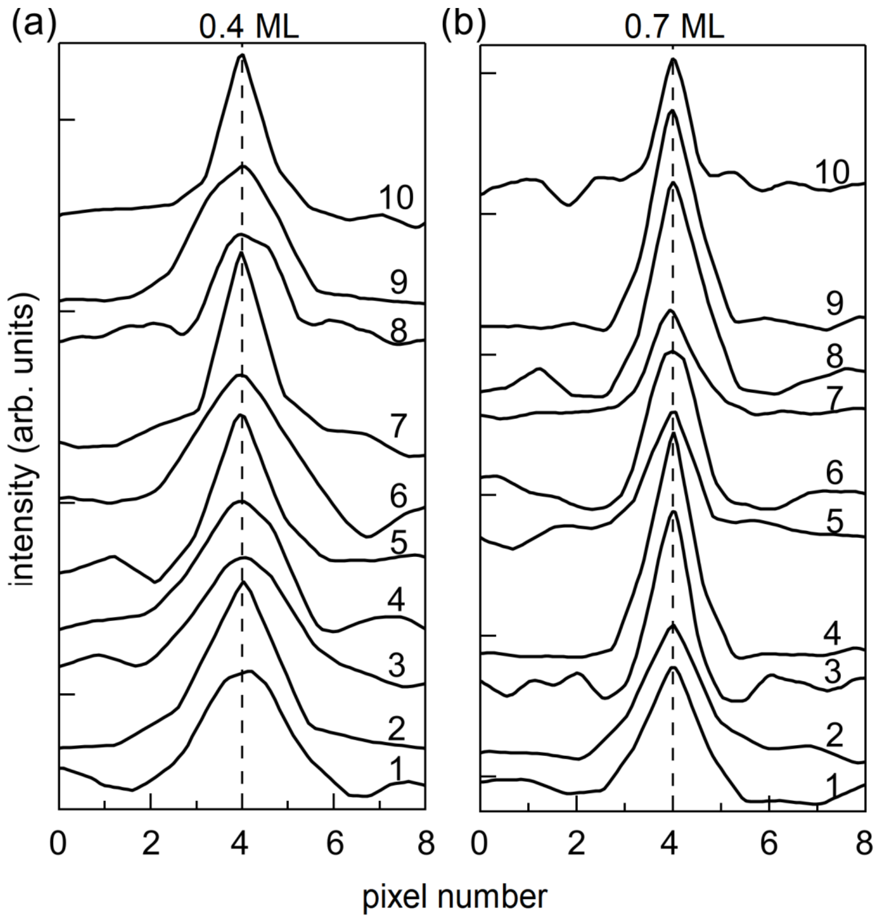


FIG. S 4. Average intensity profiles through the FFT spots numbered as 1-10 in Figs. 2(b, d) of the main text, respectively for (a) 0.4 ML, and (b) 0.7 ML coverage. The averaging is performed over 5 intensity profiles through each spot along the tangential line [e.g., the yellow dashed line in Fig. 2(b)] and at angles within $\pm 10^{\circ}$ to it.

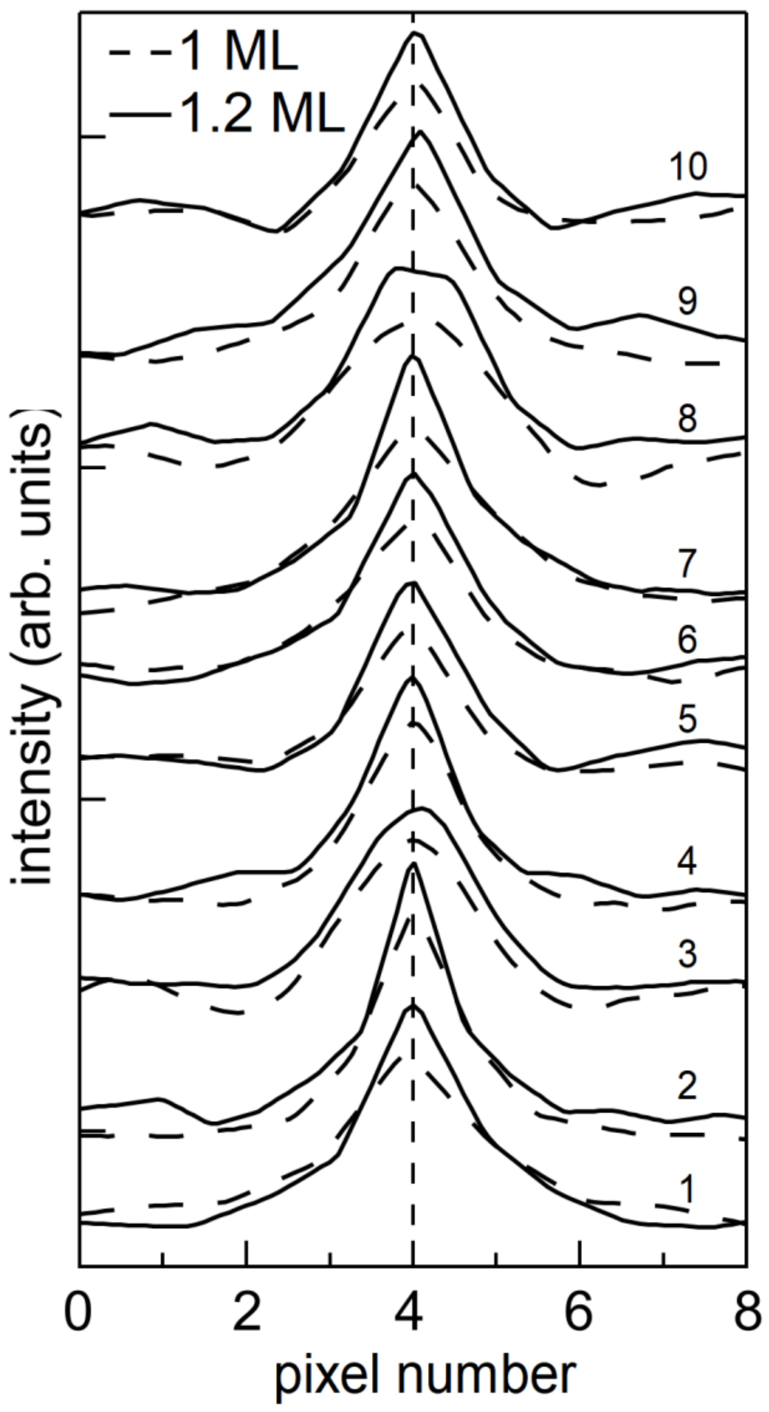


FIG. S 5. Average intensity profiles through the FFT spots in Figs. 3(b,c) of the main text. The averaging has been performed as in Fig. S4. The dashed and solid lines show the profiles for 1 ML and 1.2 ML, respectively.

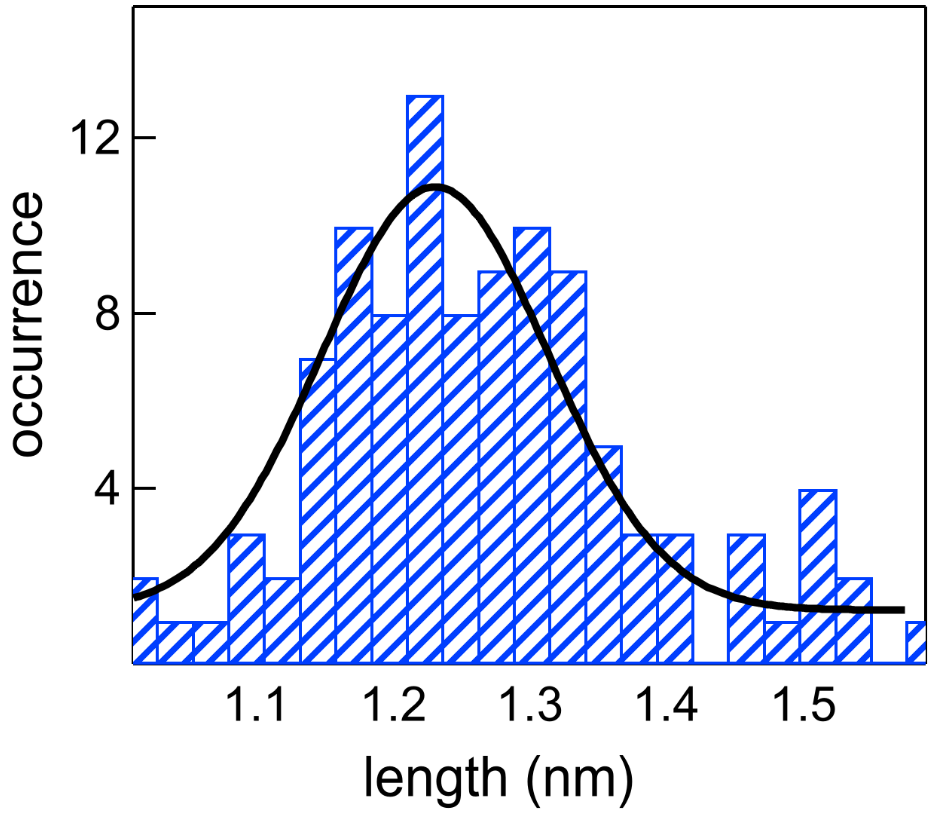


FIG. S 6. Distribution of the side length of the $\tau$-GaWF motif. The black curve represents a Gaussian fit to the distribution.

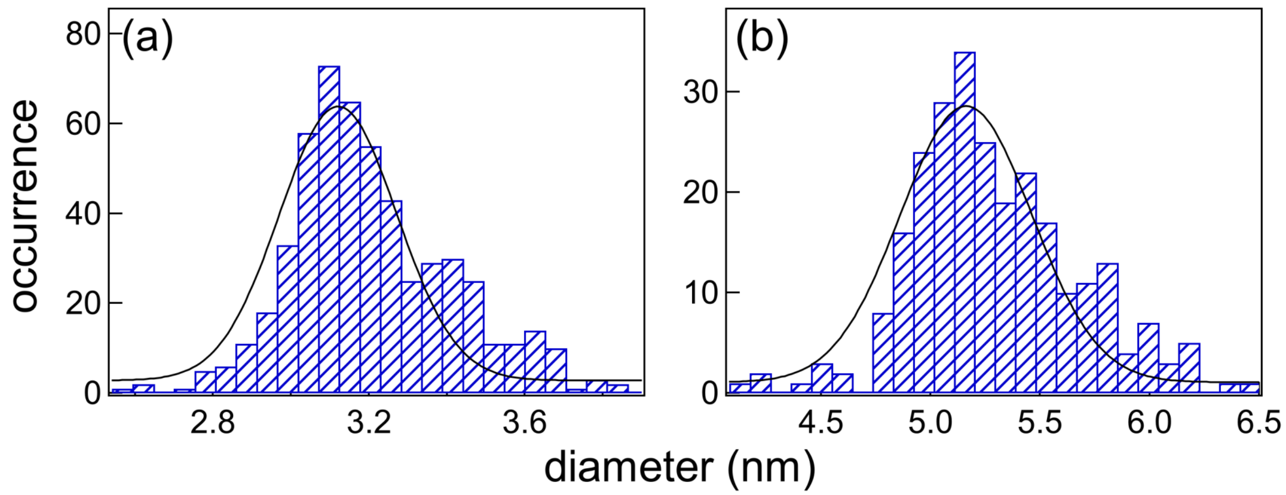


FIG. S 7. Distribution of the diameters of the (a) $\tau$-GaWF motif and (b) the ring motif. The black curve represents a Gaussian fit to the distribution.

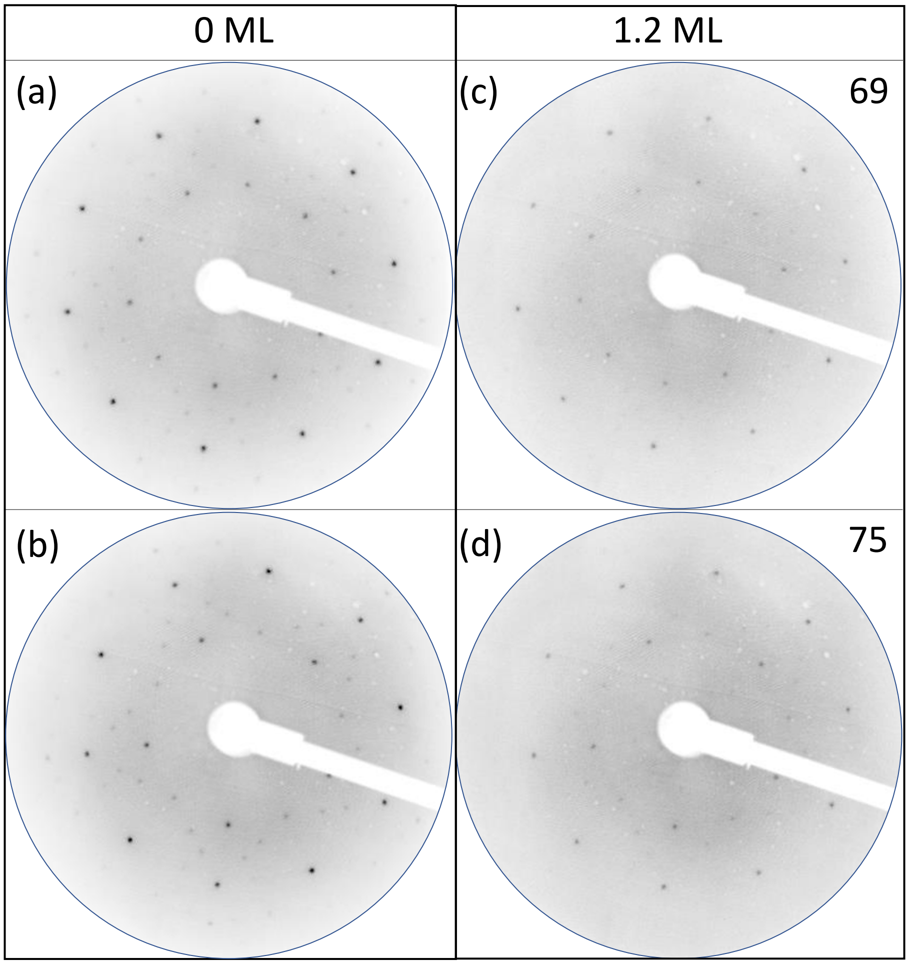


FIG. S 8. LEED patterns of (a-b) $i$-Al-Pd-Mn, (c-d) 1.2 ML Ga/$i$-Al-Pd-Mn for different $E_p$, shown at the top right corner in eV.

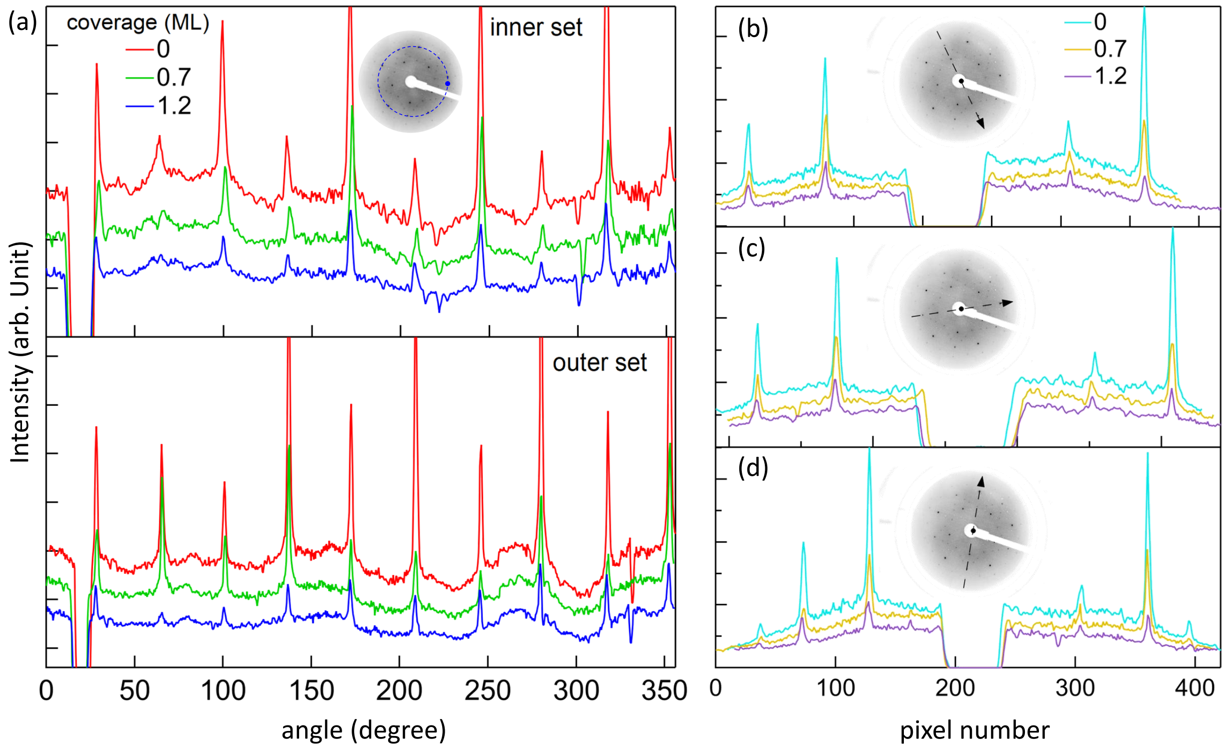


FIG. S 9. Intensity profiles of the LEED spots along a dashed circle (see inset) for 1.2 ML and 0.7 ML Ga coverage compared to the substrate (0 ML) for (a) the inner set and (b) the outer set of spots marked by blue and black arrows in Fig. 5(a) of the main text. The zero of the horizontal scale is defined by the blue dot in the inset. Intensity is zero around 20° because of the shadow of the electron source. (b-d) Intensity profiles of the LEED spots along the dashed arrow of the pattern shown in the inset for 1.2 ML and 0.7 ML Ga coverage compared to the substrate. The position of the (00) spot is indicated by a black dot.

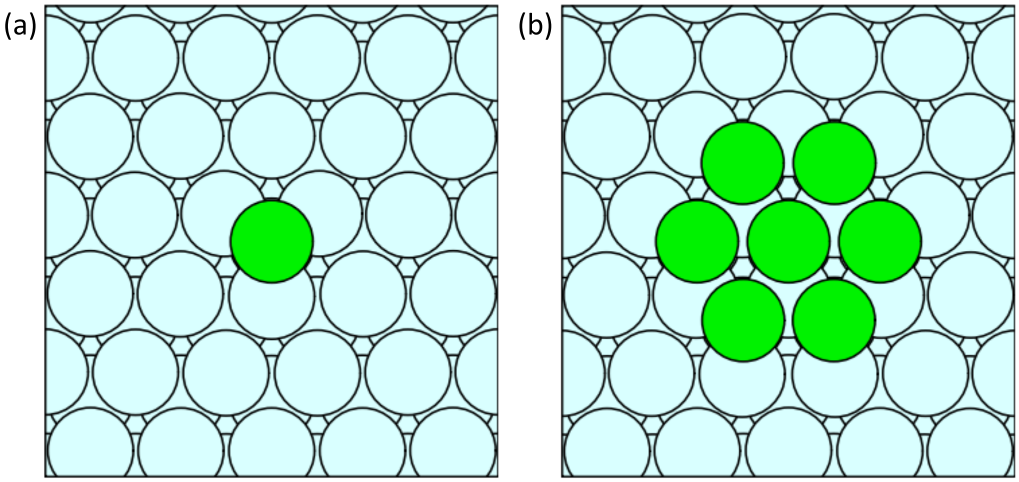


FIG. S 10. Adsorption of (a) single Ga adatom and (b) 7-atom Ga cluster on the (111) surface of Al (open circles).

[1] V. K. Singh, M. Mihalkovič, M. Krajčí, S. Sarkar, P. Sadhukhan, M. Maniraj, A. Rai, K. Pussi, D. L. Schlagel, T. A. Lograsso, A. K. Shukla, and S. R. Barman, Phys. Rev. Res. **2**, 10.1103/physrevresearch.2.013023 (2020).
